# Supplementary material for: A Two-Time-Scale Stochastic Optimization Framework with Applications in Control and Reinforcement Learning
Source: arXiv:2109.14756 source file (2024-08-23)
Supplement: Supplementary file 1 [file Supplementary_Proof_Corollary.tex]

\section{Proof Sketch of Corollary \ref{cor:LQR}}\label{sec:cor:LQR}

In this section, we briefly sketch how the analysis of Theorem \ref{thm:convergence_decision_pl} can be extended to proving Corollary \ref{cor:LQR}. We note that Assumption \ref{assump:stable_K} can be shown to imply Assumptions \ref{assump:HG_smooth}-\ref{assump:tv_bound} of the general optimization framework as discussed in Section \ref{sec:applications_lqr}.
The main difference between Theorem \ref{thm:convergence_decision_pl} and Corollary \ref{cor:LQR} is that Theorem \ref{thm:convergence_decision_pl} assumes the access to a stochastic oracle that tracks the gradient of the objective function \eqref{operator:H}, whereas in the LQR problem, we use a stochastic oracle $H$ that tracks the natural gradient\vspace{-3pt}
\begin{align*}
    \Eset_{X\sim\mu_{\theta}}[H(\theta,\omega^{\star}(\theta),X)]=\Ical_{\theta}^{-1}\nabla f(\theta),
\end{align*}
where $\Ical_{\theta}$ denotes the Fisher information matrix under $\theta$.\vspace{-5pt}
% Defining
% \begin{align*}
% \widebar{\Delta H_k} &\triangleq H(\theta_k,\omega_k,X_k)-H(\theta_k,\omega^{\star}(\theta_k),X_k),\\
% % \Gamma_H(\theta, X) &\triangleq\left\langle\nabla f(\theta),H(\theta,\omega^{\star}(\theta),X)-\mathbb{E}_{\hat{X}\sim\mu_{\theta}}[H(\theta,\omega^{\star}(\theta),\hat{X})]\right\rangle,
% \Delta H_k &\triangleq H(\theta_k,\omega^{\star}(\theta_k),X_k)-\mathbb{E}_{\hat{X}\sim\mu_{\theta_k}}[H(\theta_k,\omega^{\star}(\theta_k),\hat{X})],
% \end{align*}
By the smoothness of $f$,
% \begin{align}
%     f(\theta_{k+1})&\leq f(\theta_{k})+\langle\nabla f(\theta_k),\theta_{k+1}-\theta_k\rangle+\frac{L_f}{2}\|\theta_{k+1}-\theta_k\|^2\notag\\
%     &= f(\theta_{k})-\alpha_k\langle\nabla f(\theta_k),F(\theta_k,\omega_k,X_k)\rangle+\frac{L_f \alpha_k^2}{2}\|F(\theta_k,\omega_k,X_k)\|^2\notag\\
%     &= f(\theta_{k})-\alpha_k\langle\nabla f(\theta_k),F(\theta_k,\omega^{\star}(\theta_k),X_k)\rangle\notag\\
%     &\hspace{20pt}-\alpha_k\langle\nabla f(\theta_k),\Delta F(\theta_k, \omega_k, X_k)\rangle+\frac{L_f \alpha_k^2}{2}\|F(\theta_k,\omega_k, X_k)\|^2\notag\\
%     &= f(\theta_{k})-\alpha_k\Gamma(\theta_k,X_k)-\alpha_k\langle\nabla f(\theta_k),\mathbb{E}_{\hat{X}\sim\mu_{\theta_k}}[F(\theta_k,\omega^{\star}(\theta_k),\hat{X})]\rangle\notag\\
%     &\hspace{20pt}-\alpha_k\left\langle\nabla f(\theta_k), \Delta F(\theta_k,\omega_k, X_k)\right\rangle+\frac{L_f \alpha_k^2}{2}\|F(\theta_k,\omega_k, X_k)\|^2\notag\\
%     &= f(\theta_{k})-\alpha_k\Gamma(\theta_k,X_k)-\alpha_k\left\langle \nabla f(\theta_k),\Ical_k^{-1}\nabla f(\theta_k)\right\rangle\notag\\
%     &\hspace{20pt}-\alpha_k\left\langle\nabla f(\theta_k), \Delta F(\theta_k,\omega_k, X_k)\right\rangle+\frac{L_f \alpha_k^2}{2}\|F(\theta_k,\omega_k, X_k)\|^2\notag\\
%     &\leq f(\theta_{k})-\alpha_k\Gamma(\theta_k,X_k)-\frac{\alpha_k}{\sigma_u}\left\|\nabla f(\theta_k)\right\|^2-\alpha_k\left\langle\nabla f(\theta_k), \Delta F(\theta_k,\omega_k, X_k)\right\rangle\notag\\
%     &\hspace{20pt}+\frac{L_f \alpha_k^2}{2}\|F(\theta_k,\omega_k, X_k)\|^2,
%     \label{cor:LQR:eq1}
% \end{align}
\begin{align}
    f(\theta_{k+1})&\leq f(\theta_{k})+\langle\nabla f(\theta_k),\theta_{k+1}-\theta_k\rangle+\frac{L}{2}\|\theta_{k+1}-\theta_k\|^2\notag\\
    &= f(\theta_{k})-\alpha_k\langle\nabla f(\theta_k),H(\theta_k,\omega_k,X_k)\rangle+\frac{L \alpha_k^2}{2}\|H(\theta_k,\omega_k,X_k)\|^2\notag\\
    % &= f(\theta_{k})-\alpha_k\langle\nabla f(\theta_k),H(\theta_k,\omega^{\star}(\theta_k),X_k)\rangle\notag\\
    % &\hspace{20pt}-\alpha_k\langle\nabla f(\theta_k),\widebar{\Delta H_k}\rangle+\frac{L \alpha_k^2}{2}\|H(\theta_k,\omega_k, X_k)\|^2\notag\\
    % &= f(\theta_{k})-\alpha_k\langle\nabla f(\theta_k),\Delta H_k\rangle-\alpha_k\langle\nabla f(\theta_k),\mathbb{E}_{\hat{X}\sim\mu_{\theta_k}}[H(\theta_k,\omega^{\star}(\theta_k),\hat{X})]\rangle\notag\\
    % &\hspace{20pt}-\alpha_k\left\langle\nabla f(\theta_k), \widebar{\Delta H_k}\right\rangle+\frac{L \alpha_k^2}{2}\|H(\theta_k,\omega_k, X_k)\|^2\notag\\
    &= f(\theta_{k})-\alpha_k\langle\nabla f(\theta_k),H(\theta_k,\omega_k,X_k)-\mathbb{E}_{\hat{X}\sim\mu_{\theta_k}}[H(\theta_k,\omega^{\star}(\theta_k),\hat{X})]\rangle\notag\\
    &\hspace{20pt}-\alpha_k\left\langle \nabla f(\theta_k),\Ical_k^{-1}\nabla f(\theta_k)\right\rangle+\frac{L \alpha_k^2}{2}\|H(\theta_k,\omega_k, X_k)\|^2\notag\\
    &\leq f(\theta_{k})-\alpha_k\langle\nabla f(\theta_k),H(\theta_k,\omega_k,X_k)-\mathbb{E}_{\hat{X}\sim\mu_{\theta_k}}[H(\theta_k,\omega^{\star}(\theta_k),\hat{X})]\rangle\notag\\
    &\hspace{20pt}-\frac{\alpha_k}{\sigma_u}\left\|\nabla f(\theta_k)\right\|^2+\frac{L \alpha_k^2}{2}\|H(\theta_k,\omega_k, X_k)\|^2,
    \label{cor:LQR:eq1}
\end{align}
where the last inequality follows from the fact that the Fisher information matrix has upper bounded eigenvalue as implied by Lemma \ref{lem:bounded_sigma_SigmaK}. Comparing \eqref{cor:LQR:eq1} with \eqref{prop:pl_nonconvex:eq1} which is established under the general framework, we note that most terms of \eqref{cor:LQR:eq1} can be handled in similar manners as in Proposition \ref{prop:pl_nonconvex}. 
% we note that the terms $\left\langle\nabla f(\theta_k), \Delta H\right\rangle$, $\left\langle\nabla f(\theta_k), \widebar{\Delta H}\right\rangle$, and $\|H(\theta_k,\omega_k, X_k)\|^2$ can all be handled in similar manners as in Proposition \ref{prop:pl_nonconvex}.
The third term in \eqref{cor:LQR:eq1} has an extra scaling factor $\sigma_u^{-1}$ that does not appear in \eqref{prop:pl_nonconvex:eq1}, which essentially has to be absorbed into $\alpha_k$ and results in a scaled choice of the step size. The rest of the proof proceeds in the same way as the proof of Proposition \ref{prop:pl_nonconvex} and Theorem \ref{thm:convergence_decision_pl}.
