# Supplementary material for: A Two-Time-Scale Stochastic Optimization Framework with Applications in Control and Reinforcement Learning
Source: arXiv:2109.14756 source file (2024-08-23)
Supplement: Supplementary file 2 [file Supplementary_Proof_Lemma.tex]

\section{Proof of Lemmas}

\subsection{Proof of Lemma \ref{lem:Lambda_bound}}
Since our Markov processes are time-varying (they depend on the iterates $\theta$), one cannot directly utilize Assumption \ref{assump:markov-chain} to analyze the bias of $G$ in Algorithm \ref{Alg:two-time-scale-SGD} since the mixing time is defined for a fixed Markov chain (see Definition \ref{def:mixing_time}). To handle this difficulty, we introduce the following auxiliary Markov chain $\{\widetilde{X}_{k}\}$ generated under the decision variable $\theta_{k-\tau_k}$ starting from $X_{k-\tau_{k}}$ as follows
\begin{align}
% X_{k-\tau_k-1} \stackrel{\theta_{k-\tau_k}}{\longrightarrow}  
{X}_{k-\tau_k} \stackrel{\theta_{k-\tau_k}}{\longrightarrow}  \widetilde{X}_{k-\tau_k+1} \stackrel{\theta_{k-\tau_k}}{\longrightarrow}  \cdots \widetilde{X}_{k-1} \stackrel{\theta_{k-\tau_k}}{\longrightarrow}  \widetilde{X}_{k}.
\label{eq:def_distribution_d}
\end{align}
% and we use $d_k$ to denote the distribution of $\widetilde{X}_{k}$. 
% Thus, one can apply Assumption \ref{assump:markov-chain} to $\{\widetilde{X}_{k}\}$. 
For clarity, recall the time-varying Markov processes $\{X_k\}$ generated by Algorithm~\ref{Alg:two-time-scale-SGD}
\begin{align*}
% X_{k-\tau_k-1} \stackrel{\theta_{k-\tau_k}}{\longrightarrow} 
X_{k-\tau_k} \stackrel{\theta_{k-\tau_k+1}}{\longrightarrow} X_{k-\tau_k+1} \stackrel{\theta_{k-\tau_k+2}}{\longrightarrow} \cdots \stackrel{\theta_{k-1}}{\longrightarrow} X_{k-1} \stackrel{\theta_{k}}{\longrightarrow} X_{k}.
\end{align*}
Recall $z_{k} = \omega_{k} - \omega^{\star}(\theta_{k})$. We define the following quantities
% defined over $X_{k}$ and $\widetilde{X}_{k}$
\begin{align*}
    &T_{1}=\mathbb{E}[\langle\omega_{k}-\omega_{k-\tau_k}, G(\theta_k,\omega_k,X_k)-\mathbb{E}_{\hat{X}\sim\mu_{\theta_k}}[G(\theta_k,\omega_k,\hat{X})]\rangle],\notag\\
    &T_{2}=\mathbb{E}[\langle\omega^{\star}(\theta_{k-\tau_k})-\omega^{\star}(\theta_k), G(\theta_k,\omega_k,X_k)-\mathbb{E}_{\hat{X}\sim\mu_{\theta_k}}[G(\theta_k,\omega_k,\hat{X})]\rangle],\notag\\
    &T_{3}=\mathbb{E}[\langle z_{k-\tau_k},G(\theta_k,\omega_k,X_k)-G(\theta_{k-\tau_k},\omega_{k-\tau_k},X_k)\rangle],\notag\\
    &T_{4}=\mathbb{E}[\langle z_{k-\tau_k}, G(\theta_{k-\tau_k},\omega_{k-\tau_k},X_k)-G(\theta_{k-\tau_k},\omega_{k-\tau_k}, \widetilde{X}_k)\rangle],\notag\\
    &T_{5}=\mathbb{E}[\langle z_{k-\tau_k}, G(\theta_{k-\tau_k},\omega_{k-\tau_k}, \widetilde{X}_k)-\mathbb{E}_{\bar{X}\sim \mu_{\theta_{k-\tau_k}}}[G(\theta_{k-\tau_k},\omega_{k-\tau_k},\bar{X})]\rangle],\notag\\
    &T_{6}=\mathbb{E}[\langle z_{k-\tau_k}, \mathbb{E}_{\bar{X}\sim \mu_{\theta_{k-\tau_k}}}[G(\theta_{k-\tau_k},\omega_{k-\tau_k},\bar{X})]-\mathbb{E}_{\hat{X}\sim\mu_{\theta_k}}[G(\theta_{k-\tau_k},\omega_{k-\tau_k},\hat{X})]\rangle],\notag\\
    &T_{7}=\mathbb{E}[\langle z_{k-\tau_k}, \mathbb{E}_{\hat{X}\sim\mu_{\theta_k}}[G(\theta_{k-\tau_k},\omega_{k-\tau_k},\hat{X})]-\mathbb{E}_{\hat{X}\sim\mu_{\theta_k}}[G(\theta_{k},\omega_{k},\hat{X})]\rangle].
\end{align*}
It is easy to see that
\begin{align}
    \mathbb{E}[\langle\omega_k-\omega^{\star}(\theta_k), \Delta G_k\rangle] 
    % &= \mathbb{E}\big[\langle\omega_k-\omega^{\star}(\theta_k), G(\theta_k,\omega_k,X_k)-\mathbb{E}_{\hat{X}\sim\mu_{\theta_k}}[G(\theta_k,\omega_k,\hat{X})]\rangle\big]\notag\\
    % &=\mathbb{E}\big[\big\langle\omega_k-\omega^{\star}(\theta_k), G(\theta_k,\omega_k,X_k)-\mathbb{E}_{\hat{X}\sim\mu_{\theta_k}}[G(\theta_k,\omega_k,\hat{X})]\big\rangle\big]\notag\\
    % &=\mathbb{E}\big[\big\langle\omega_k-\omega_{k-\tau_k}, G(\theta_k,\omega_k,X_k)-\mathbb{E}_{\hat{X}\sim\mu_{\theta_k}}[G(\theta_k,\omega_k,\hat{X})]\big\rangle\big]\notag\\
    % &\hspace{20pt}+\mathbb{E}\big[\big\langle\omega^{\star}(\theta_{k-\tau_k})-\omega^{\star}(\theta_k), G(\theta_k,\omega_k,X_k)-\mathbb{E}_{\hat{X}\sim\mu_{\theta_k}}[G(\theta_k,\omega_k,\hat{X})]\big\rangle\big]\notag\\
    % &\hspace{20pt}+\mathbb{E}\big[\big\langle\omega_{k-\tau_k}-\omega^{\star}(\theta_{k-\tau_k}), G(\theta_k,\omega_k,X_k)-\mathbb{E}_{\hat{X}\sim\mu_{\theta_k}}[G(\theta_k,\omega_k,\hat{X})]\big\rangle\big]\notag\\
    &=T_{1}+T_{2}+T_{3}+T_{4}+T_{5}+T_{6}+T_{7}.\label{lem:Lambda_bound:Eq0}
\end{align}
We analyze the terms of \eqref{lem:Lambda_bound:Eq0} individually. First, using \eqref{eq:G_affinelybounded_D} we consider
\begin{align*}
    T_{1}&\leq \mathbb{E}[\|\omega_k-\omega_{k-\tau_k}\|\|G(\theta_k,\omega_k,X_k)-\mathbb{E}_{\hat{X}\sim\mu_{\theta_k}}[G(\theta_k,\omega_k,\hat{X})]\|]\notag\\
    &\leq \mathbb{E}\big[\|\omega_k-\omega_{k-\tau_k}\|\left(\|G(\theta_k,\omega_k,X_k)\|+\|\mathbb{E}_{\hat{X}\sim\mu_{\theta_k}}[G(\theta_k,\omega_k,\hat{X})]\|\right)\big]\notag\\
    &\leq 2D\mathbb{E}\big[\|\omega_k-\omega_{k-\tau_k}\|\left(\|\theta_k\|+\|\omega_k\|+1\right)\big],
\end{align*}
which combined with Lemma \ref{lem:omega_k-omega_k-tau} gives
\begin{align}
    T_{1} &\leq 6D^2\beta_{k-\tau_k}\tau_k\mathbb{E}\big[\left(\|\theta_k\|+\|\omega_k\|+1\right)^2\big]\leq 18D^2\beta_{k-\tau_k}\tau_k\mathbb{E}\big[\|\theta_k\|^2+\|\omega_k\|^2+1\big].\label{lem:Lambda_bound:eq1a}    
\end{align}
Similarly, using Assumption \ref{assump:Lipschitz_omega} we bound $T_2$ as
\begin{align}
    &T_{2}\leq \mathbb{E}[\|\omega^{\star}(\theta_{k-\tau_k})-\omega^{\star}(\theta_k)\|\| G(\theta_k,\omega_k,X_k)-\mathbb{E}_{\hat{X}\sim\mu_{\theta_k}}[G(\theta_k,\omega_k,\hat{X})]\|]\notag\\
    % &\leq 2D\mathbb{E}\big[\|\omega^{\star}(\theta_{k-\tau_k})-\omega^{\star}(\theta_k)\|\left(\|\theta_k\|+\|\omega_k\|+1\right)\big]\notag\\
    &\leq 2DL\mathbb{E}[\|\theta_k\hspace{-2pt}-\hspace{-2pt}\theta_{k-\tau_k}\|\left(\|\theta_k\|\hspace{-2pt}+\hspace{-2pt}\|\omega_k\|\hspace{-2pt}+\hspace{-2pt}1\right)]\hspace{-2pt}=\hspace{-2pt} 2DL\mathbb{E}\big[\big\|\hspace{-4pt}\sum_{t=k-\tau_{k}}^{k-1}\hspace{-5pt}\alpha_{t}H(\theta_{t},\omega_{t},H_{t})\big\|\hspace{-1pt}(\|\theta_k\|\hspace{-2pt}+\hspace{-2pt}\|\omega_k\|\hspace{-2pt}+\hspace{-2pt}1)\hspace{-1pt}\big]\notag\\
    &\leq 2DB L\tau_k\alpha_{k-\tau_k}\mathbb{E}[\|\theta_k\|+\|\omega_k\|+1]\leq DB L\tau_k\alpha_{k-\tau_k} \mathbb{E}[\|\theta_k\|^2+\|\omega_k\|^2+4],\label{lem:Lambda_bound:eq1b}    
\end{align}
where the equality is due to \eqref{alg:update_theta}, the third inequality follows from \eqref{assump:H_bounded}, and the last inequality applies $2c\leq c^2+1$ for any scalar $c$. Using Assumption \ref{assump:HG_smooth}, \eqref{assump:H_bounded}, and Lemma \ref{lem:omega_k-omega_k-tau} we analyze $T_3$ in a similar way
\begin{align}
T_{3} &\leq\mathbb{E}\big[\|z_{k-\tau_k}\|\|G(\theta_k,\omega_k,X_k)-G(\theta_{k-\tau_k},\omega_{k-\tau_k},X_k)\|\big]\notag\\
&\leq L\mathbb{E}\big[\|z_{k-\tau_k}\|\left(\|\theta_k-\theta_{k-\tau_k}\|+\|\omega_k-\omega_{k-\tau_k}\|\right)\big]\notag\\
&\leq L B\tau_k\alpha_{k-\tau_k}\mathbb{E}\big[\|z_{k-\tau_k}\|\big]+3L D\beta_{k-\tau_k}\tau_k\mathbb{E}\big[\|z_{k-\tau_k}\|\left(\|\omega_k\|+\|\theta_{k}\|+1\right)\big]\notag\\
&\leq \frac{L B\tau_k\alpha_{k-\tau_k}}{2}\mathbb{E}\big[\|z_{k-\tau_k}\|^2+1\big]+\frac{3L D\beta_{k-\tau_k}\tau_k}{2}\mathbb{E}\big[\|z_{k-\tau_k}\|^2+\left(\|\omega_k\|+\|\theta_{k}\|+1\right)^2\big]\notag\\
&\leq 2L D\tau_k\beta_{k-\tau_k}\mathbb{E}\big[\|z_{k-\tau_k}\|^2\big]\hspace{-2pt}+\hspace{-2pt}\frac{9L D\tau_k\beta_{k-\tau_k}}{2}\mathbb{E}\big[\|\omega_k\|^2\hspace{-2pt}+\hspace{-2pt}\|\theta_{k}\|^2\big]\hspace{-2pt}+\hspace{-2pt}5L D\tau_k\beta_{k-\tau_k},\label{lem:Lambda_bound:eq1c}    
\end{align}
where the last inequality follows from $\alpha_k\leq\beta_k$ for all $k\geq 0$. To analyze $T_{4}$, we utilize the law of total expectation: given $\Fcal\subseteq\Fcal'$ and a random variable $X$ we have $\Eset[X\mid\Fcal] = \Eset[\Eset[X\mid\Fcal']\mid\Fcal]$.   

Let $\Fcal_k$ be $\Fcal_k=\{X_0,\ldots,X_k,\theta_0,\ldots,\theta_k,\omega_0,...,\omega_k\}$,
and for convenience we denote
\[p_{k}(x) = P(X_{k} = x\mid\Fcal_{k-1})\quad  \text{and}\quad  \tilde{p}_{k}(x) = P(\widetilde{X}_{k} = x\mid\Fcal_{k-1}).\]
Then, by the Cauchy-Schwarz inequality we have
\begin{align*}
    &\mathbb{E}[\langle z_{k-\tau_k}, G(\theta_{k-\tau_k},\omega_{k-\tau_k},X_k)-G(\theta_{k-\tau_k},\omega_{k-\tau_k}, \widetilde{X}_k)\rangle\mid\Fcal_{k-\tau_k}]\notag\\
    % &=\left\langle z_{k-\tau_k}, \mathbb{E}\big[G(\theta_{k-\tau_k},\omega_{k-\tau_k},X_k)-G(\theta_{k-\tau_k},\omega_{k-\tau_k}, \widetilde{X}_k)\mid\Fcal_{k-\tau_k}\big]\right\rangle\notag\\
    &\leq\left\|z_{k-\tau_k}\right\| \left\|\mathbb{E}\big[ G(\theta_{k-\tau_k},\omega_{k-\tau_k},X_k)-G(\theta_{k-\tau_k},\omega_{k-\tau_k}, \widetilde{X}_k)\mid\Fcal_{k-\tau_k}\big]\right\|\notag\\
    % &=\left\|z_{k-\tau_k}\right\| \left\|\mathbb{E}\left[\Eset\left[ G(\theta_{k-\tau_k},\omega_{k-\tau_k},X_k)-G(\theta_{k-\tau_k},\omega_{k-\tau_k}, \widetilde{X}_k)\mid \Fcal_{k-1}\right] \mid\Fcal_{k-\tau_k}\right]\right\|\notag\\
    &=\left\|z_{k-\tau_k}\right\| \Big\|\Eset\Big[\int_{\Xcal}G(\theta_{k-\tau_k},\omega_{k-\tau_k},x)(p_{k}(x)-\tilde{p}_{k}(x))dx \mid\Fcal_{k-\tau_{k}}\Big]\Big\|\notag\\
    &\leq 2D\left\|z_{k-\tau_k}\right\|(\|\theta_{k-\tau_k}\|+\|\omega_{k-\tau_k}\|+1)\big\|\Eset\big[d_{TV}(p_{k}(\cdot),\tilde{p}_{k}(\cdot))\mid \Fcal_{k-\tau_k}\big],
\end{align*}
where the last inequality uses the definition of the TV distance in \eqref{eq:TV_def}. Recursively applying Assumption \ref{assump:tv_bound}, we obtain from the preceding relation
\begin{align}
&\mathbb{E}\big[\left\langle z_{k-\tau_k}, G(\theta_{k-\tau_k},\omega_{k-\tau_k},X_k)-G(\theta_{k-\tau_k},\omega_{k-\tau_k}, \widetilde{X}_k)\right\rangle\mid\Fcal_{k-\tau_k}\big]\notag\\
&\leq  2D\hspace{-2pt}\left\|z_{k-\tau_k}\right\|\hspace{-1pt}(\|\theta_{k-\tau_k}\|\hspace{-2pt}+\hspace{-2pt}\|\omega_{k-\tau_k}\|\hspace{-2.5pt}+\hspace{-2.5pt}1)\big\|\Eset\big[d_{TV}(p_{k-1}(\cdot),\tilde{p}_{k-1}(\cdot)) \hspace{-2pt}+\hspace{-2pt} L\|\theta_{k-1}\hspace{-2pt}-\hspace{-2pt}\theta_{k-\tau_k}\|\hspace{-1pt}\mid\hspace{-2pt}\Fcal_{k-\tau_{k}}\big]\notag\\
&\leq  2LD\left\|z_{k-\tau_k}\right\|(\|\theta_{k-\tau_k}\|+\|\omega_{k-\tau_k}\|+1)\sum_{t=k-\tau_{\alpha_{k}}}^{k-1}\Eset\big[\|\theta_{t}-\theta_{k-\tau_k}\|\mid\Fcal_{k-\tau_k}\big]\notag, 
\end{align}
where the last inequality we use $d_{TV}(p_{k-\tau_k}(\cdot),\tilde{p}_{k-\tau_k}(\cdot)) = 0$. Since the operator $H$ is bounded (assumed in \eqref{assump:H_bounded}) we have
\begin{align*}
    \sum_{t=k-\tau_k+1}^{k-1} \hspace{-7pt}\|\theta_t\hspace{-2pt}-\hspace{-2pt}\theta_{k-\tau_k}\|]\hspace{-2pt}\leq\hspace{-5pt} \sum_{t=k-\tau_k+1}^{k}\sum_{t'=k-\tau_k}^{t-1} \hspace{-7pt}\|\theta_{t'+1}\hspace{-2pt}-\hspace{-2pt}\theta_{t'}\|]\hspace{-2pt}\leq \hspace{-6pt}\sum_{t=k-\tau_k+1}^{k}\sum_{t'=k-\tau_k}^{t-1}\hspace{-7pt}B\alpha_{k-\tau_k}\leq B\tau_k^2\alpha_{k-\tau_k},
\end{align*}
which we substitute into the equation above and take the expectation on both sides
\begin{align}
    T_{4}&\leq 2DBL\tau_k^2\alpha_{k-\tau_k}\mathbb{E}\big[\left\|z_{k-\tau_k}\right\|(\|\theta_{k-\tau_k}\|+\|\omega_{k-\tau_k}\|+1)\big].
\end{align}
On the other hand, we consider
\begin{align}
    &\left\|z_{k-\tau_k}\right\|(\|\theta_{k-\tau_k}\|+\|\omega_{k-\tau_k}\|+1)\notag\\
    % &\leq \left\|z_{k-\tau_k}\right\|(\|\theta_{k}\|+\|\theta_{k}-\theta_{k-\tau_k}\|+\|\omega_{k}\|+\|\omega_{k}-\omega_{k-\tau_k}\|+1)\notag\\
    &\leq \left\|z_{k-\tau_k}\right\|(\|\theta_k\|+B\tau_k\alpha_{k-\tau_k}+\|\omega_{k}\|+\|\omega_{k}-\omega_{k-\tau_k}\|+1)\notag\\
    &\leq \left\|z_{k-\tau_k}\right\|(\|\theta_k\|+\|\omega_{k}\|+\frac{1}{2}(\|\omega_k\|+\|\theta_k\|+1)+\frac{7}{6})\notag\\
    &\leq 2\left\|z_{k-\tau_k}\right\|(\|\theta_k\|+\|\omega_{k}\|+1)\leq \left\|z_{k-\tau_k}\right\|^2+(\|\theta_k\|+\|\omega_{k}\|+1)^2\notag\\
    &\leq \left\|z_{k-\tau_k}\right\|^2+3(\|\theta_k\|^2+\|\omega_{k}\|^2+1),\label{lem:Lambda_bound:eq1d1}
\end{align}
where the second inequality uses the step size condition $B\tau_k\alpha_{k-\tau_k}\leq\frac{1}{6}$ and Lemma \ref{lem:omega_k-omega_k-tau}. Using \eqref{lem:Lambda_bound:eq1d1} in the equation above, we have
\begin{align}
    T_{4}&\leq DBL\tau_k^2\alpha_{k-\tau_k}\mathbb{E}\big[\left\|z_{k-\tau_k}\right\|^2\big]+3DBL\tau_k^2\alpha_{k-\tau_k}\mathbb{E}\big[\|\theta_k\|^2+\|\omega_{k}\|^2+1\big].\label{lem:Lambda_bound:eq1d}
\end{align}
Next, we bound $T_{5}$ using Assumption \ref{assump:markov-chain}
\begin{align*}
T_{5} &=
    \Eset\Big[\mathbb{E}\big[\left\langle z_{k-\tau_k}, G(\theta_{k-\tau_k},\omega_{k-\tau_k}, \widetilde{X}_k)-\mathbb{E}_{\bar{X}\sim \mu_{\theta_{k-\tau_k}}}[G(\theta_{k-\tau_k},\omega_{k-\tau_k},\bar{X})]\right\rangle\mid\Fcal_{k-\tau_k}\big]\Big]\notag\\
    % &=\Eset\Big[\left\langle z_{k-\tau_k}, \mathbb{E}\big[G(\theta_{k-\tau_k},\omega_{k-\tau_k}, \widetilde{X}_k)-\mathbb{E}_{\bar{X}\sim \mu_{\theta_{k-\tau_k}}}[G(\theta_{k-\tau_k},\omega_{k-\tau_k},\bar{X})]\mid\Fcal_{k-\tau_k}\big]\right\rangle\Big]\notag\\
    &\leq \Eset[\|z_{k-\tau_k}\| \big\|\mathbb{E}[G(\theta_{k-\tau_k},\omega_{k-\tau_k}, \widetilde{X}_k)-\mathbb{E}_{\bar{X}\sim \mu_{\theta_{k-\tau_k}}}[G(\theta_{k-\tau_k},\omega_{k-\tau_k},\bar{X})]\mid\Fcal_{k-\tau_k}]\big\|]\notag\\
    &\leq D\Eset[\|z_{k-\tau_k}\|(\|\theta_{k-\tau_k}\|+\|\omega_{k-\tau_k}\|+1)\mathbb{E}[d_{TV}(\widetilde{p}_k(\cdot),\mu_{\theta_{k-\tau_k}})\mid\Fcal_{k-\tau_k}]]\notag\\
    &\leq D\alpha_{k}\Eset[\|z_{k-\tau_k}\|(\|\theta_{k-\tau_k}\|+\|\omega_{k-\tau_k}\|+1)]\notag\\
    &\leq D\alpha_{k}\mathbb{E}[\|z_{k-\tau_k}\|^2\big]+3D\alpha_{k}\mathbb{E}\big[\|\theta_k\|^2+\|\omega_k\|^2+1],
    % &\leq D\|z_{k-\tau_k}\|(\|\theta_{k-\tau_k}\|+\|\omega_{k-\tau_k}\|+1)m\rho^{\tau_k}.
\end{align*}
where the last inequality is due to \eqref{lem:Lambda_bound:eq1d1}. 
We next consider $T_{6}$,
\begin{align*}
    &\mathbb{E}\big[\left\langle z_{k-\tau_k}, \mathbb{E}_{\bar{X}\sim \mu_{\theta_{k-\tau_k}}}[G(\theta_{k-\tau_k},\omega_{k-\tau_k},\bar{X})]-\mathbb{E}_{\hat{X}\sim\mu_{\theta_k}}[G(\theta_{k-\tau_k},\omega_{k-\tau_k},\hat{X})]\right\rangle\mid\Fcal_{k-\tau_k}\big]\notag\\
    % &= \left\langle z_{k-\tau_k}, \mathbb{E}\big[\hspace{-1pt}\mathbb{E}_{\bar{X}\sim \mu_{\theta_{k-\tau_k}}}\hspace{-2pt}[G(\theta_{k-\tau_k},\omega_{k-\tau_k},\bar{X})]\hspace{-1pt}-\mathbb{E}_{\hat{X}\sim\mu_{\theta_k}}[G(\theta_{k-\tau_k},\omega_{k-\tau_k},\hat{X})]\mid\Fcal_{k-\tau_k}\big]\right\rangle\notag\\
    &\leq \left\|z_{k-\tau_k}\right\| \left\|\mathbb{E}\big[\hspace{-1pt}\mathbb{E}_{\bar{X}\sim \mu_{\theta_{k-\tau_k}}}\hspace{-3pt}[G(\theta_{k-\tau_k},\omega_{k-\tau_k},\bar{X})]-\mathbb{E}_{\hat{X}\sim\mu_{\theta_k}}\hspace{-2pt}[G(\theta_{k-\tau_k},\omega_{k-\tau_k},\hat{X})]\mid\Fcal_{k-\tau_k}\big]\right\|\notag\\
    &\leq \left\|z_{k-\tau_k}\right\|D(\|\theta_{k-\tau_k}\|+\|\omega_{k-\tau_k}\|+1) \mathbb{E}\big[d_{TV}(\mu_{\theta_k},\mu_{\theta_{k-\tau_k}})\mid\Fcal_{k-\tau_k}\big]\notag\\
    &\leq D L\left\|z_{k-\tau_k}\right\|(\|\theta_{k-\tau_k}\|+\|\omega_{k-\tau_k}\|+1) \mathbb{E}[\|\theta_k-\theta_{k-\tau_k}\|\mid\Fcal_{k-\tau_k}]\notag\\
    &\leq D B L\tau_k\alpha_{k-\tau_k}\left\|z_{k-\tau_k}\right\|(\|\theta_{k-\tau_k}\|+\|\omega_{k-\tau_k}\|+1),
\end{align*}
where the third inequality uses \eqref{assump:tv_bound:eq2} in Assumption \ref{assump:tv_bound}. Again, we can employ \eqref{lem:Lambda_bound:eq1d1}
\begin{align*}
    T_{6}&\leq DBL\tau_k\alpha_{k-\tau_k}\mathbb{E}\big[\|z_{k-\tau_k}\|^2\big]+3DBL\tau_k\alpha_{k-\tau_k}\mathbb{E}\big[\|\theta_k\|^2+\|\omega_k\|^2+1\big].
\end{align*}
Finally, using the Cauchy-Schwarz inequality and the Lipschitz continuity of $G$,
\begin{align*}
    &T_{7}
    \leq\mathbb{E}\big[\left\|z_{k-\tau_k}\right\|\left\| \mathbb{E}_{\hat{X}\sim\mu_{\theta_k}}[G(\theta_{k-\tau_k},\omega_{k-\tau_k},\hat{X})-G(\theta_{k},\omega_{k},\hat{X})]\right\|\big]\notag\\
    &\leq L\mathbb{E}\big[\left\|z_{k-\tau_k}\right\|\left(\|\theta_k-\theta_{k-\tau_k}\|+\|\omega_k-\omega_{k-\tau_k}\|\right)\big]\notag\\
    &\leq\mathbb{E}\big[\frac{L (B\hspace{-2pt}+\hspace{-2pt}3D)\tau_k\beta_{k-\tau_k}}{2}\|z_{k-\tau_k}\|^2\hspace{-2pt}+\hspace{-2pt}\frac{9L D\tau_k\beta_{k-\tau_k}}{2}\|\omega_k\|^2\hspace{-2pt}+\hspace{-2pt}\|\theta_{k}\|^2\big]+\frac{L (B\hspace{-2pt}+\hspace{-2pt}9D)\tau_k\beta_{k-\tau_k}}{2},
    % \label{lem:Lambda_bound:eq1f}
\end{align*}
where the derivation of the last inequality is identical to that of $T_{3}$. 
Finally, plugging the bound on $T_1$-$T_7$
% \eqref{lem:Lambda_bound:eq1a}--\eqref{lem:Lambda_bound:eq1f}
in \eqref{lem:Lambda_bound:Eq0} and simplifying the terms using the relations $\alpha_k\leq\beta_k$, $\tau_k\geq 1$ leads to the claimed result.
